# Supplementary material for: What Matters In On-Policy Reinforcement Learning? A Large-Scale Empirical Study
Source: arXiv:2006.05990 source file (2020-06-10)
Supplement: Supplementary file 1 [file dummy_appendix.tex]

\clearpage
\section{Experiment E1}
\subsection{Design}
For each of the 5 environments, we sampled X choice configurations where we sampled the following choices independently and uniformly from the following ranges:
\begin{itemize}
    \item Choice 1: \{Option 1, Option 2\}
    \item Choice 2: \{asdf, aaaa\}
    \begin{itemize}
        \item For the case ``Choice 2 = asdf'', we further sampled the sub-choices:
        \begin{itemize}
        \item Subchoice 1: \{option 1, Option 2\}
        
        \item Subchoice 1: \{option 1, Option 2\}
        \end{itemize}
        
        \item For the case ``Choice 2 = aaaa'', we further sampled the sub-choices:
        \begin{itemize}
        \item Subchoice 3: \{option 1, Option 2\}
        \item Subchoice 4: \{option 1, Option 2\}
        \end{itemize}
    \end{itemize}
\end{itemize}
All the other choices were set to the default values as described in Section~\ref{sec:default_settings}.

For each of the sampled choice configurations, we train Y agents with different random seeds and compute the performance metric as described in Section~\ref{sec:performance}.

\subsection{Results}
We report aggregate statistics of the experiment in Table~\ref{tab:e1_overview} as well as training curves in Figure~\ref{fig:e1_training_curves}.
For each of the investigated choices in this experiment, we further provide a per-choice analysis in Figures~\ref{fig:e1_choice_first}-\ref{fig:e1_choice_last}

\begin{table}[ht]
\begin{center}
\caption{Performance quantiles across choice configurations for experiment E1}
\label{tab:e1_overview}
  \begin{tabular}{lrrrrr}
\toprule
{} &                    Ant-v1 &        HalfCheetah-v1 &                 Hopper-v1 &               Humanoid-v1 &               Walker2d-v1 \\
\midrule
0.9     &                   3553.36 &               2679.13 &                   1553.64 &                   3985.46 &                   921.279 \\
0.95    &                   4101.55 &               3396.36 &                   1970.56 &                    4731.1 &                   1235.64 \\
0.99    &                   4887.02 &               4629.17 &                   2419.24 &                   5787.76 &                   2068.24 \\
max     &                    5984.2 &               6490.19 &                   2949.66 &                   7504.26 &                   3340.92 \\
\bottomrule
\end{tabular}
\end{center}
\end{table}

\begin{figure}[ht]
\begin{center}
    \centerline{\includegraphics[width=0.45\textwidth]{13759846/perf__gin_study_design_choice_value_action_postprocessing.pdf}\includegraphics[width=0.45\textwidth]{13759846/frequency__gin_study_design_choice_value_action_postprocessing.pdf}}
    \caption{Analysis of choice ``Action postprocessing'' in E1: 95th percentile of performance scores conditioned on choice (left) and distribution of choices in top 5\% of configurations (right).}
    \label{fig:e1_choice_sdfs}
\end{center}
\end{figure}

\clearpage
